# Supplementary material for: VISTA: Triplet-Supervised Video Style Transfer with Diffusion Transformers
Source: arXiv:2605.17312 source file (2026-05-17)
Supplement: Supplementary file 1 [file X_suppl.tex]

\section{LLM Usage}
In preparing this work, we used LLMs as an assistive tool. Specifically, LLMs (e.g., ChatGPT) were employed to refine the clarity and readability of manuscript drafts through language polishing. Importantly, all research ideas, methodology design, experimental implementation, and analysis were conceived and conducted by the authors. The LLMs were not used for generating research hypotheses, designing experiments, or interpreting results. The authors take full responsibility for the content of this paper.

\section{Video Results}
Video generation results, including qualitative comparisons with baseline methods, are provided in the supplementary material archive.
The archive contains full-resolution videos for all evaluated methods and benchmarks.
We encourage readers to refer to the supplementary videos for a detailed visual comparison of stylization quality, motion consistency, and temporal stability.
